# Supplementary material for: Influence of long range forces on the transition states and dynamics of NaCl ion-pair dissociation in water
Source: arXiv:2110.05646 ancillary file (2021-10-11)
Supplement: Supplementary file 1 [file supplement.pdf]

# Supplementary Material: Influence of long range forces on the transition states and dynamics of NaCl ion-pair dissociation in water

**Wang, Zhao, Weeks and Tiwary**

## I. SIMULATION DETAILS

The LAMMPS package is modified to include $v_0$ term (see Eq. 1 in main text) that arises from Gaussian-truncated charges.[1] Alternatively, $v_0$ can be realized by tabulating the potential without modifying the source code. For the full system, Coulomb interactions are evaluated using particle-particle particle-mesh method, with a real space cutoff of 9.8 Å and a precision of $10^{-6}$. For the CGT model, all the interactions, including $v_0$ and Lennard-Jones potentials, are short-ranged and computed by direct summation within the cutoff of 9.8 Å. The Nose-Hoover thermostat[2] and barostat[3], with damping constants of 0.1 and 1.0 ps, respectively, are utilized to implement the isothermal isobaric (NPT) ensemble at $T = 300$ K and $P = 1$ atm with a time step of 1 fs. The pressure correction due to truncated Coulomb interactions is applied to the CGT model.[4]

For each system, a 100 ns long equilibrium trajectory is generated for further kinetic analyses. We generated a 100 ns long trajectory because the potential of mean force and the mean first passage time of the ion-pair dissociation are hard to converge. However, we also found that the analysis of SPIB generally requires much less data, and a 25 ns trajectory ($\sim$ 20 association/dissociation events) is enough for SPIB to generate converged results.

## II. ORDER PARAMETERS FOR THE ION PAIR SYSTEM

By referring to Ref. 5, we select 13 order parameters (OPs) in total. All of these 13 OPs are widely used and easy to calculate.

- (1): Ion-pair distance, $r_{ion}$ – The distance between the sodium cation and chloride anion.

- (2)–(5): Ion coordination numbers, $N_{Na,1}$, $N_{Na,2}$, $N_{Cl,1}$, $N_{Cl,2}$ – The number of water molecules within the 1th/2nd radial shell around Na/Cl was counted

$$N_{is} = \sum_{w} f_{iws} \tag{1}$$

where the sum is over all water molecules and the continuous indicator function is

$$f_{iws} = \frac{1 - \tanh\left[a(r_{iw} - b_{is})\right]}{2}. \tag{2}$$

The subscripts $i$, $w$ and $s$ refer to an ion, a water molecule, and solvation shell, respectively. The ion-water distance $r_{iw}$ is to the oxygen atom when calculating $Na^+$ coordination and to the closest hydrogen atom when calculating $Cl^-$ coordination. The parameters are $b_{Na,1} = 3.25$ Å, $b_{Cl,1} = 3.1$ Å, $b_{Na,2} = b_{Cl,2} = 5.75$ Å, $a = 3$.

- (6)–(7): Ion-pair coordination number, $N_{ip1}$, $N_{ip2}$ – The number of waters coordinated to the ion pair is

$$N_{ips} = \sum_w \max\left(f_{Na,ws}, f_{Cl,ws}\right) \tag{3}$$

- (8): Number of bridging waters, $N_B$ - The number of waters jointly coordinated to the first shell of both ions simultaneously is

$$N_B = \sum_w \min\left(f_{Na,w1}, f_{Cl,w1}\right) \tag{4}$$

- (9)–(13): Interionic water density, $\rho_{i0}$, $\rho_{i1}$, $\rho_{i2}$, $\rho_{i3}$, $\rho_{i4}$ – The number density of water molecules between the two ions was calculated by summing over a Gaussian indicator function

$$\rho_{ik} = \frac{1}{(2\pi\sigma_k^2)^{3/2}} \sum_w \exp\left(-\frac{(r_w - r_{mid})^2}{2\sigma_k^2}\right) \tag{5}$$

where $r_{mid}$ is the midpoint between the ions, $r_w$ is simply the position of the oxygen atom of the w-th water molecule. There are 5 options for $\sigma_k$: $3.7Å$, $r_{ion}$, $r_{ion}/2$, $r_{ion}/3$, $r_{ion}/4$.

## III. DETAILS OF STATE PREDICTIVE INFORMATION BOTTLENECK

For a given unbiased trajectory $\{\boldsymbol{X}^1, \cdots, \boldsymbol{X}^{M+s}\}$ and its corresponding state labels $\{\boldsymbol{y}^1, \cdots, \boldsymbol{y}^{M+s}\}$ with large enough $M$, the objective function of SPIB can be formulated as:

$$\mathcal{L} \approx \frac{1}{M \cdot L} \sum_{n=1}^{M} \sum_{l=1}^{L} \Big[\log q_\theta(\boldsymbol{y}^{n+s}|\boldsymbol{z}^{(n,l)}) - \beta \log \frac{p_\theta(\boldsymbol{z}^{(n,l)}|\boldsymbol{X}^n)}{r_\theta(\boldsymbol{z}^{(n,l)})}\Big] \tag{6}$$

where $\boldsymbol{z}^{(n,l)}$ is sampled from $p_\theta(\boldsymbol{z}|\boldsymbol{X}^n)$ and the time interval between $\boldsymbol{X}^n$ and $\boldsymbol{X}^{n+s}$ is the time delay $\Delta t$. Based on rate-distortion theory,[6,7] the first term in Eq. 6 can be interpreted as the distortion, which measures the ability of our representation to predict the desired

target, while the second term can be interpreted as the rate, which measures the number of bits per data sample to be transmitted. Reducing the rate will limit the ability of $\boldsymbol{z}$ to predict the target, increasing the distortion. Therefore, maximizing this objective function results in a competition between the rate and the distortion. Such a trade-off can be controlled by the hyper-parameter $\beta$. In principle, an ideal $\beta$ will utilize every byte transmitted with maximum efficiency to predict the target. In this work, we chose the turning point of the Rate-Distortion plot as the optimum $\beta$ in order to obtain a maximally informative representation. However, we also found that as long as $\beta$ is not too large, its value will not have a big impact on our results.

In SPIB, the trajectory $\{\boldsymbol{X}^n\}$ is usually expressed in terms of many order parameters or features, while the state labels $\{\boldsymbol{y}^n\}$ are mutually exclusive and expressed in terms of one-hot vectors, i.e. a binary vector with a single high (1) bit and all the others low (0). To implement this we use a deep feed forward neural network with softmax outputs in our decoder $q_\theta(\boldsymbol{y}|\boldsymbol{z})$.

$$\log q_\theta(\boldsymbol{y}^{n+s}|\boldsymbol{z}^n) = \sum_{i=1}^{D} y_i^{n+s} \log \mathcal{D}_i(\boldsymbol{z}^n;\theta) \tag{7}$$

where the state label $\boldsymbol{y}$ is a one-hot vector of $D$ dimensions and the decoder function $\boldsymbol{\mathcal{D}}$ is the $D$-dimensional softmax output of a neural network.

Given that we expect the learnt RC should demarcate between different metastable states, it is natural to assume a multi-modal distribution for the prior $r_\theta(\boldsymbol{z})$. In our algorithm, we employ the variational mixture of posteriors prior (VampPrior) to obtain such a multi-modal prior distribution.[8] Here, the approximate prior $r_\theta(\boldsymbol{z})$ is a weighted mixture of different posteriors $p_\theta(\boldsymbol{z}|\boldsymbol{X})$ with pseudo-inputs $\{\boldsymbol{u}^k\}_{k=1}^K$ in lieu of $\boldsymbol{X}$:

$$r_\theta(\boldsymbol{z}) = \sum_{k=1}^{K} \omega_k \; p_\theta(\boldsymbol{z}|\boldsymbol{u}^k) \tag{8}$$

where $K$ is the number of pseudo-inputs, $\boldsymbol{u}^k$ is a vector which has the same dimension as input $\boldsymbol{X}$, and $\omega_k$ represents the weight of $p_\theta(\boldsymbol{z}|\boldsymbol{u}^k)$ under the constraint $\sum_k \omega_k = 1$. The pseudo-inputs $\{\boldsymbol{u}^k\}$ and weights $\{\omega_k\}$ can be thought of the parameters of the prior, which are learned through backpropagation of the objective function (Eq. 6). In principle, the number of pseudo-inputs should be equal to the number of metastable states in the system. In practical settings however for real-world applications to complex molecular systems, the number of metastable states is unknown *a priori*. To deal with such cases, the simple and

powerful solution is to choose a large enough $K$ making the prior more flexible.

Finally, for simplicity, we take the encoder $p_\theta(\boldsymbol{z}|\boldsymbol{X})$ in Eq. 8 as a deep neural network with a multivariate Gaussian output:

$$\log p_\theta(\boldsymbol{z}^n|\boldsymbol{X}^n) = \log \mathcal{N}(\boldsymbol{z}^n; \boldsymbol{\mu}, \boldsymbol{\sigma} I) \tag{9}$$

where the mean $\boldsymbol{\mu}$ and variance $\boldsymbol{\sigma}^2$ are outputs of a neural network whose input is $\boldsymbol{X}^n$. $I$ is the identity matrix. Then we can use the reparameterization trick[9] to write $p_\theta(\boldsymbol{z}^n|\boldsymbol{X}^n)d\boldsymbol{z}^n = p(\boldsymbol{\epsilon})d\boldsymbol{\epsilon}$ and $\boldsymbol{z}^n = \boldsymbol{\mu}(\boldsymbol{X}^n) + \boldsymbol{\sigma}(\boldsymbol{X}^n) \cdot \boldsymbol{\epsilon} = \boldsymbol{\mathcal{E}}(\boldsymbol{X}^n, \boldsymbol{\epsilon}; \theta)$, where $\boldsymbol{\epsilon} \sim \mathcal{N}(0, I)$ and the encoder function $\boldsymbol{\mathcal{E}}$ is a deterministic nonlinear function parameterized by a neural network.

With this set-up, we now introduce a simple iterative scheme that is at the heart of our SPIB approach, as it allows us to learn the number and location of states on the fly with minimal human intervention. We start with an arbitrary set of labels $\{1, ..., D\}$ for the system, where both the number and location of labels are some initial guess. If the system initiated from a certain high-dimensional configuration $\boldsymbol{X}$ has the largest probability to be found after time delay $\Delta t$ in some state $i$ from these initial labels, then the label of the configuration $\boldsymbol{X}$ will be refined and updated to state $i$. The central idea is that if one configuration was located at state $i$ at a certain time, then after time delay $\Delta t$, it should still have the largest probability to be found at state $i$, since $\Delta t$ is much shorter than the typical escape time from a metastable state.

We can denote the deterministic output of SPIB as $\hat{\boldsymbol{y}} = \boldsymbol{K}(\boldsymbol{X}; \Delta t, \theta)$, whose component $K_i(\boldsymbol{X}; \Delta t)$ can be interpreted as the probability that the system starting from $\boldsymbol{X}$ will be found in state $i$ after a time delay $\Delta t$. Then a set of new state labels can be generated by:

$$h_i(\boldsymbol{X}) = \begin{cases} 1 \ (i = \underset{j}{\operatorname{argmax}}\ K_j(\boldsymbol{X}; \Delta t, \theta)) \\ 0 \ (\text{otherwise}) \end{cases} \quad \text{for } i = 1, \ldots, D. \tag{10}$$

This label refinement step might very well lead to null assignments for some of the labels we started with, as shown in the main text. The whole algorithm is summarized through Alg. 1 and Supplementary Fig. 1.

## IV. NEURAL NETWORK ARCHITECTURE AND TRAINING

In this paper, both the encoder and decoder are nonlinear and parameterized by fully connected neural networks with two hidden layers as shown in Supplementary Fig. 2. Each

**Algorithm 1** SPIB

**Input:** a long unbiased trajectory $\{\boldsymbol{X}^n\}$, a set of initial state labels $\{\boldsymbol{y}^n\}$, RC dimensionality $d$, the number of pseudo-inputs $K$, time delay $\Delta t$

**repeat**

  **repeat**

    Sample a minibatch $\{\boldsymbol{X}^n\}$ and $\{\boldsymbol{y}^n\}$

    Calculate the objective function $\mathcal{L}$

    Update the neural network parameters $\theta$, pseudo-inputs $\{\boldsymbol{u}^k\}_{k=1}^K$, pseudo-weights $\{\omega_k\}_{k=1}^K$

  **until** the prediction of new state labels are converged

  Update the state labels $\{\boldsymbol{y}^n\}$ by Eq. 10

**until** convergence of RC, state-transition density, and state labels

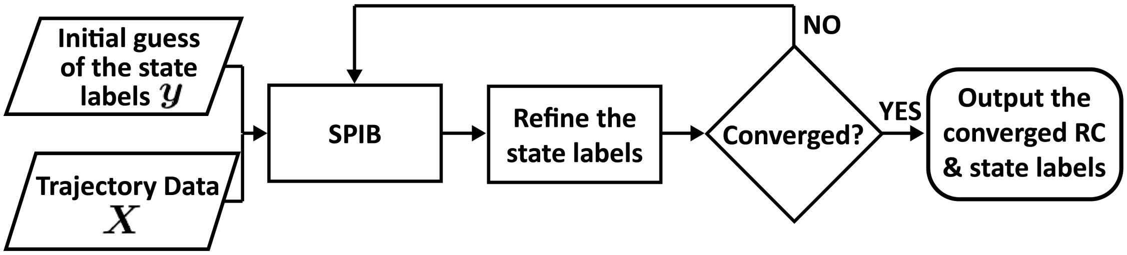


**Supplementary Figure 1:** A flowchart illustrating SPIB.

hidden layer in both the encoder and decoder has 32 nodes. All these hidden layers use a rectified linear unit (ReLU) as the activation function.

The networks were trained using the Adam optimizer[10]. To speed up the convergence during each iteration of label refinement, we started from a large learning rate of 0.01, and reduced the learning rate by a factor of 10 every 5 epochs until the prediction of new state labels are converged. This scheme led to better convergence of the state labels compared to using a high learning rate throughout. We found the state labels are harder to converge for small batches, while the algorithm seems easier to get stuck in the local minimum/maximum for large batches. A batch size of 8192 used here is a good compromise.

## V. METASTABLE STATES ANALYSIS

Here we set the RC dimension $d = 2$, the number of pseudo-inputs $K = 10$ and the dimension of initial state labels $D = 10$. In other words, here we have deliberately taken $K$ and $D$ to be arbitrarily large relative to the true number of metastable states. As shown in Supplementary Fig. 3(a,b), we choose $\beta = 0.001$ to let the 2D RC only contain the important information. However, Supplementary Fig. 3(c) illustrates that the robustness of the fractional population to the choice of $\beta$. We also want to point out that the state labels learned by SPIB are very robust to the random seeds, with very small relative standard deviations of the state populations ($< 0.0005$) over 10 random repetitions (Supplementary Fig. 3(d)).

As discussed in the main text, the time delay $\Delta t$ plays an important role in the simplification of the learning process. A time delay $\Delta t = 0$ is tantamount to ignoring the dynamics completely and simply clustering the input configuration into different states, while $\Delta t > 0$ can filter out all the fast modes, helping us ignore unnecessary details of the dynamical processes. The same time-dependent results are also obtained for CGT system (Supplementary Fig. 4). The larger the time delay is, the more coarse-grained representation we can obtain. Moreover, we also need to point out that although our results depend on the selection of

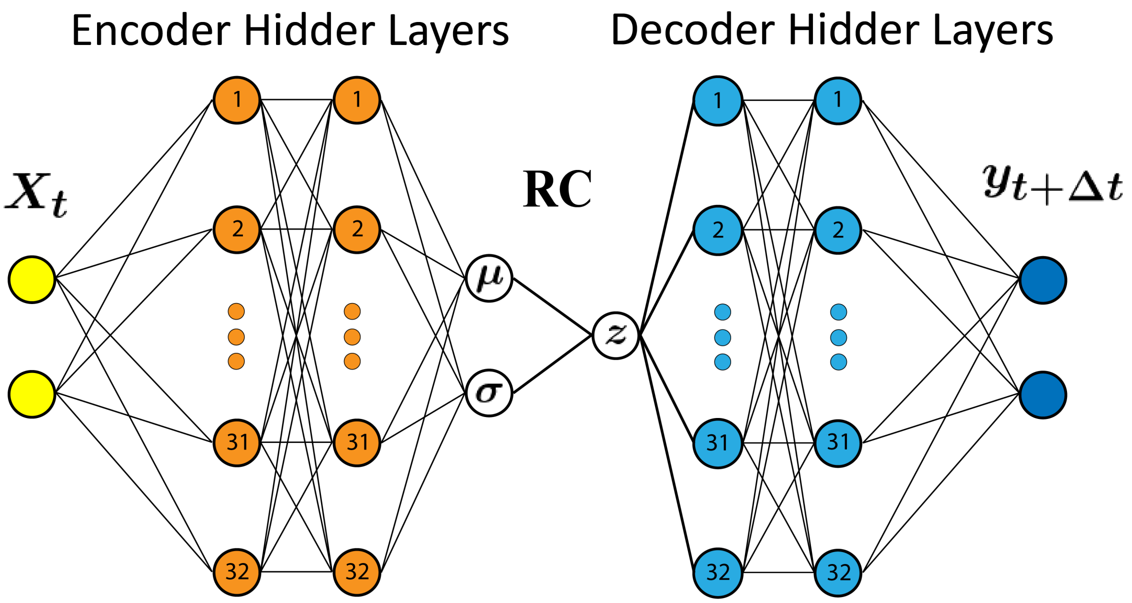


**Supplementary Figure 2:** Network architecture used for SPIB. Generalizing Ref. 11, both the encoder and decoder are nonlinear deep neural networks.

time delay, they are in fact still very robust to changes of $\Delta t$. Supplementary Fig. 5 shows a broad range of $\Delta t$ can result in the same discrete-state representation.

The four metastable states learned with the time delay $\Delta t = 0.4$ *ps* are projected to different order parameters shown in Supplementary Fig. 7 & 8. The implied timescales are shown in Supplementary Fig. 6.

Besides the long-lived intermediate state, two more intermediate states can also be identified using a smaller time delay $\Delta t = 0.1$ *ps* as shown in Supplementary Fig. 9. In Supplementary Fig. 10, the implied time scale shows that these two intermediate states (state 5 and state 7) are really very transient (about 0.1 *ps*). From the results, we can clearly see these intermediate states including the long-lived one (state 4) are located just near the transition states that we are interested in. Thus their existence can largely explain the why even after the system pass through the transition states, it can still recross back to the contact state. However, we also need to indicate that the escape time of those transient intermediate states may be underestimated as these intermediate state may not be accurately characterized by our existing order parameters.

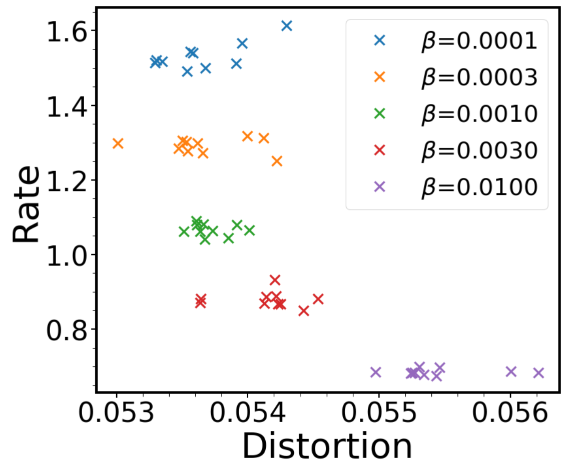


**(a)** Train

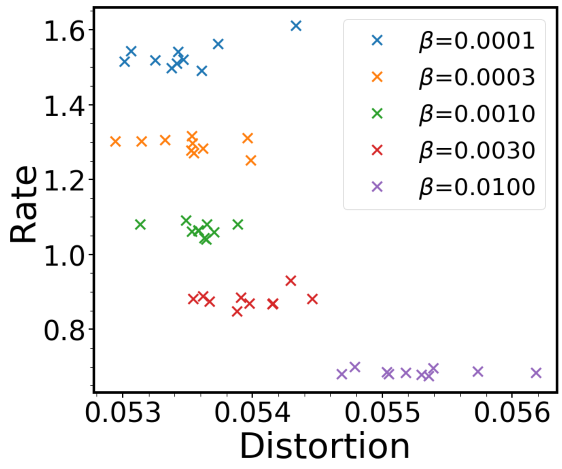


**(b)** Test

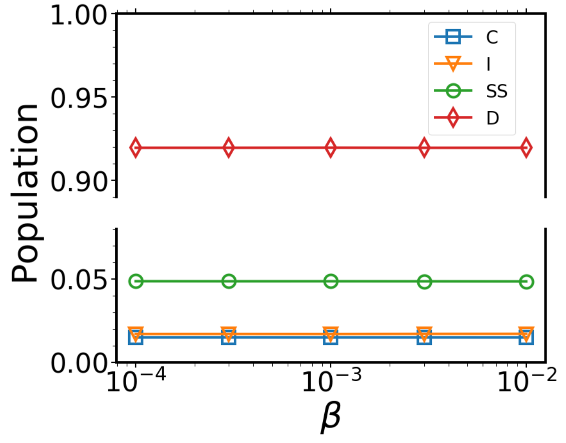


**(c)**

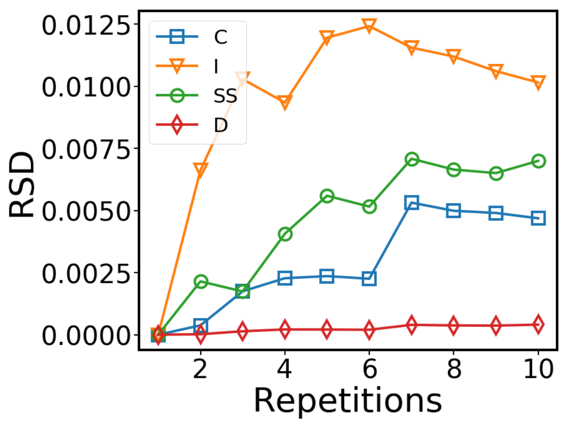


**(d)**

**Supplementary Figure 3:** The Rate-Distortion plot with the time delay $\Delta t = 0.4$ $ps$ over 10 random repetitions (a,b). The turning point of the plot ($\beta = 0.001$) is selected to obtain the most informative 2D RC in the main text. Four metastable states are obtained with the time delay $\Delta t = 0.4$ $ps$: the contact state (C), the intermediate state (I), the solvent separated state (SS) and the dissociated state (D). (c) shows the robustness of the fractional population to the choice of $\beta$ with the time delay $\Delta t = 0.4$ $ps$. (d) illustrates that the relative standard deviations of the state populations are small ($< 2\%$) over the 10 random repetitions.

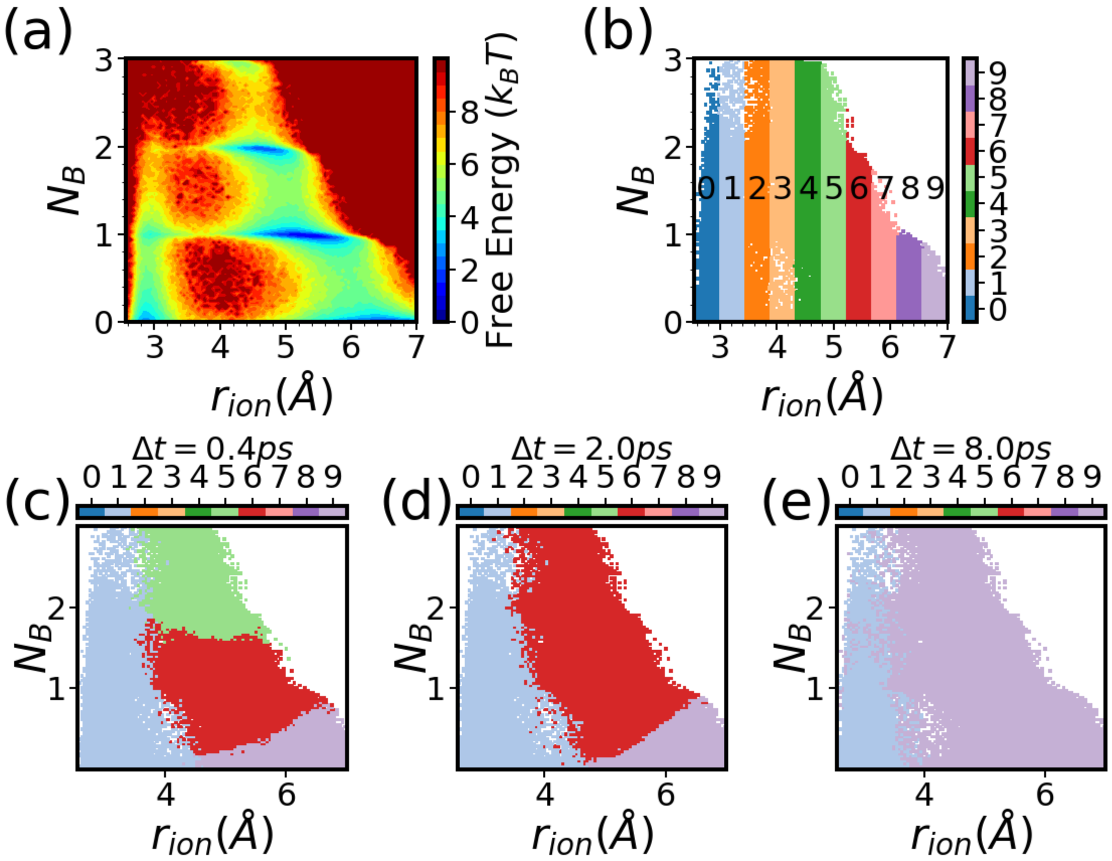


**Supplementary Figure 4:** The free energy surface (a) and the time delay dependent discrete-state representation (b-e) for the CGT system projected onto coordinates $r_{ion}$ and $N_B$. The initial state labels are shown in (b), while the converged the state labels for different time delays are presented in (c-e). The state labels are learned using the time delay $\Delta t = 0.4ps$ (b), $\Delta t = 2.0ps$ (c), and $\Delta t = 10.0ps$ (d) respectively. The color (or state label) in each grid corresponds only to the state label with highest fraction of samples for the respective grid point.

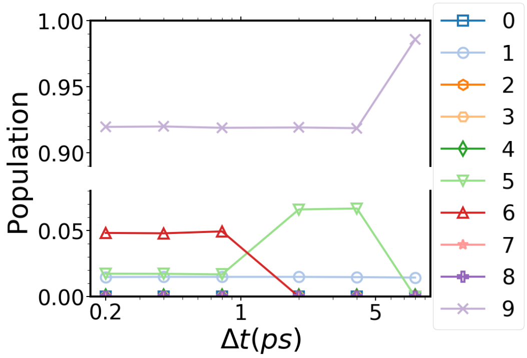


**(a)** Full

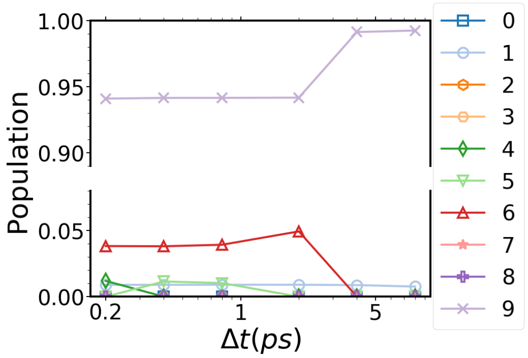


**(b)** CGT

**Supplementary Figure 5:** The robustness of SPIB to the change to time delay $\Delta t$ can be seen by plotting the fractional population of different states ($f_i = \sum_{j=1}^{N} y_i^j / N \quad for$ $i = 0, \cdots, 9$). With different time resolutions (or time delays $\Delta t$), the system is coarse grained into four states, three states and two states.

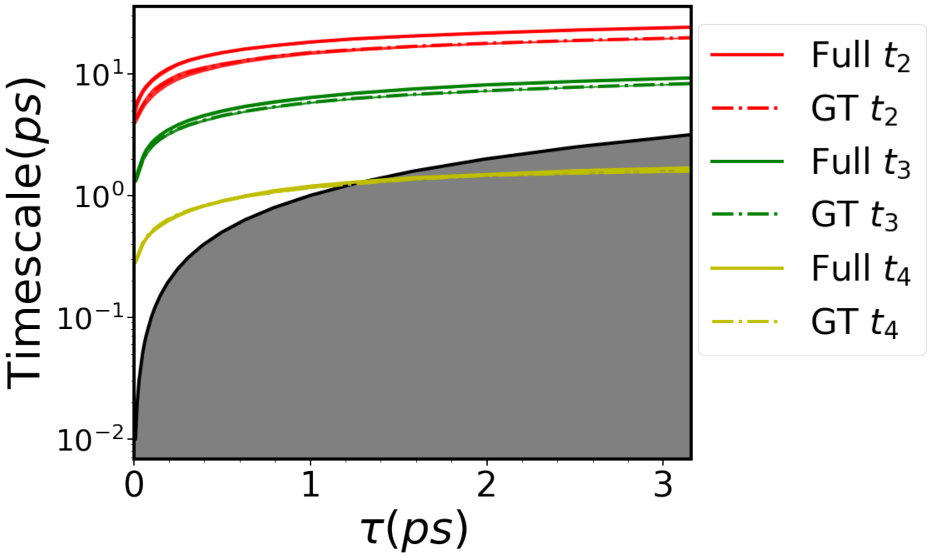


**Supplementary Figure 6:** Implied timescales computed from the four state Markov model obtained by SPIB for the full system (solid lines) and the CGT system (dashed lines). The standard deviation over 10 random training runs is reported. The grey area under the black line represents the timescale that is smaller than the lag time $\tau$.

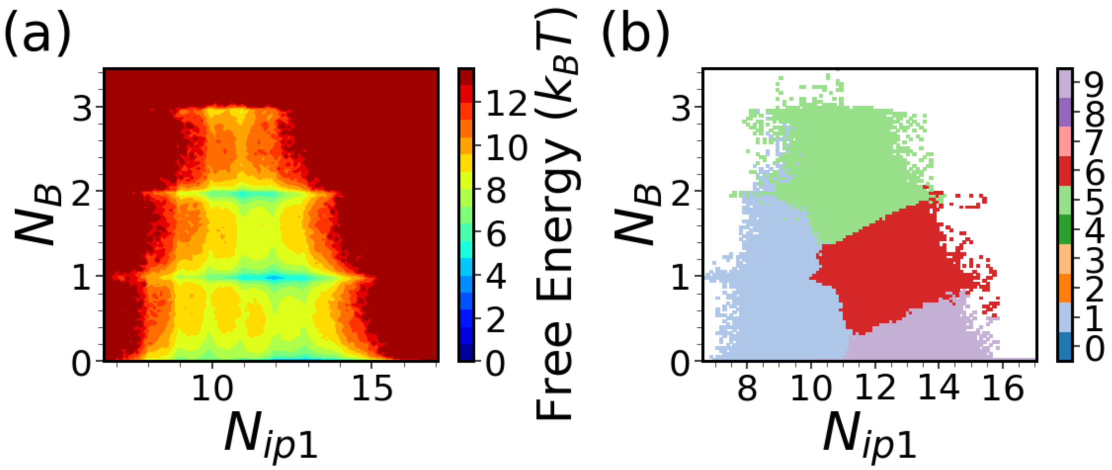


**Supplementary Figure 7:** The free energy surface (a) and the four metastable states identified by SPIB (b) for the full system projected onto coordinates $N_{ip1}$ and $N_B$. $N_{ip1}$ is the total number of water molecules in the first solvation shell of $Na^+$ and $Cl^-$, and $N_B$ is the number of bridging water molecules. The color (or state label) in each grid corresponds only to the state label with highest fraction of samples for the respective grid point.

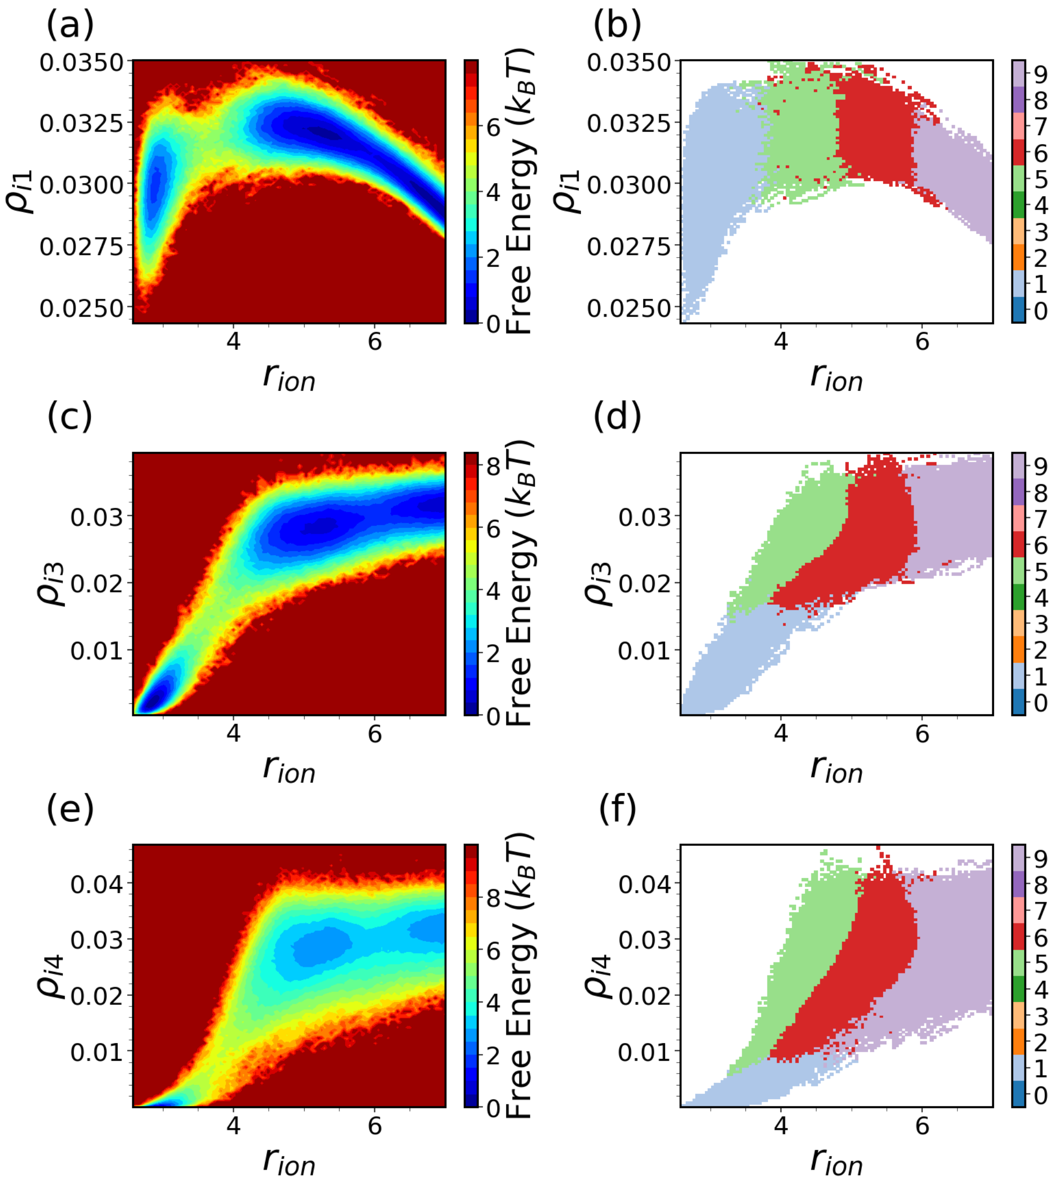


**Supplementary Figure 8:** The free energy surface (a,c,e) and the four metastable states identified by SPIB (b,d,f) for the full system projected onto different coordinates. $\rho_{i1}$, $\rho_{i3}$ and $\rho_{i4}$ all represent the interionic water density just with different resolution $\sigma$. The color (or state label) in each grid corresponds only to the state label with highest fraction of samples for the respective grid point.

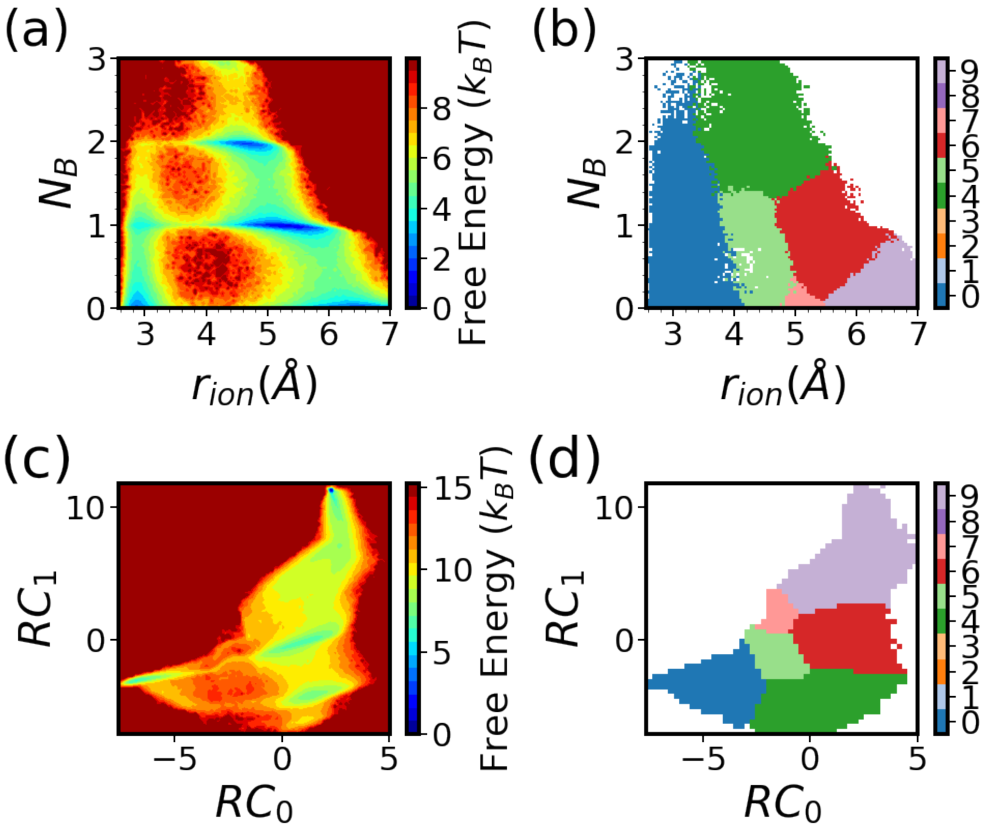


**Supplementary Figure 9:** The free energy surface (a,c) and the discrete-state representation (b,d) for the full system with $\Delta t = 0.1\ ps$. Two more intermediate states (state 5 and state 7) can be found.

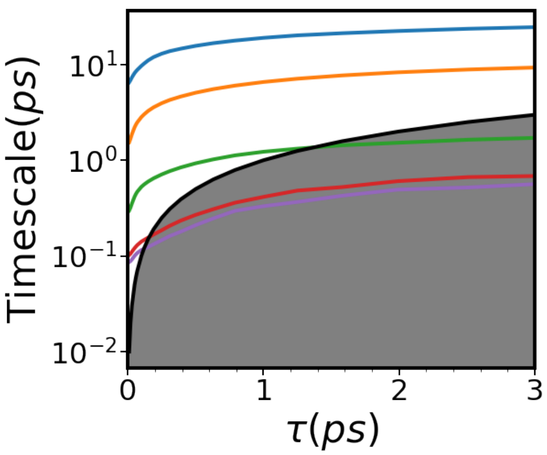


**(a)**

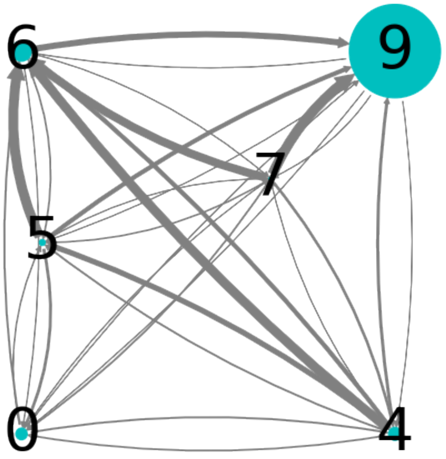


**(b)**

**Supplementary Figure 10:** The implied timescales (a) and corresponding the network representation of the transition probability matrix (b) computed from the six states Markov model obtained by SPIB for the full system with $\Delta t = 0.1$ $ps$.

## VI. TRANSITION STATE ENSEMBLE ANALYSIS

The existence of the long-lived intermediate state identified in the last subsection makes it unreasonable to directly study the transitions between the contact state and the solvent-shared state while ignoring all the intermediate states between them. Thus, we still take a four-state representation to describe the dissociation process and define the transition state ensemble as the configurations whose transition probability to the contact state is 0.5.

To test whether SPIB can identify the correct transition states, we did a traditional, detailed committor analysis and obtained the reference committor. For this we launched 20 5-ps trajectories with random initial Maxwell-Boltzmann velocities for each configuration identified as the transition state by SPIB, and then calculated their committor function $P_B$ based on the fraction of trajectories reaching $B$ ($r_{ion} > 5.0$Å) prior to $A$ ($r_{ion} < 2.9$Å). For a good RC, the committor probability distribution should be characterized by a single peak centered at 0.5. However, the obtained committor probability distribution shown in Fig. 11(a) suggested that the 13 configuration-based OPs seem not enough to identify the TSE accurately. Following the suggestion given by Ref. 5, we then introduced the accelerations of the original 13 configuration-based OPs as 13 new OPs. Accelerations were calculated by central finite difference using configurations $h = \pm 0.2ps$. After including the acceleration OPs, the new transition state ensemble identified by SPIB is shown in Supplementary Fig. 13. We did find that the new committor probability distribution is significantly improved (Supplementary Fig. 11(b)). Supplementary Fig. 12 has illustrated why the acceleration OPs or the generalized forces (e.g. $\ddot{r}_{ion}$) can be used to improve the prediction of TSE. However, we also find their ability to predict TSE is relatively sensitive to the choice of the spacing $h$. Only a generalized force that persist for intermediate times can be used to tighten the committor distribution. This finding is consistent with the previous work.[12] Interestingly, as suggested by this work, the short-ranged forces will dominate this ion pair dissociation process, thus it's promising to identify a "short-ranged force" OP which only depends on the local property of the system in the future.

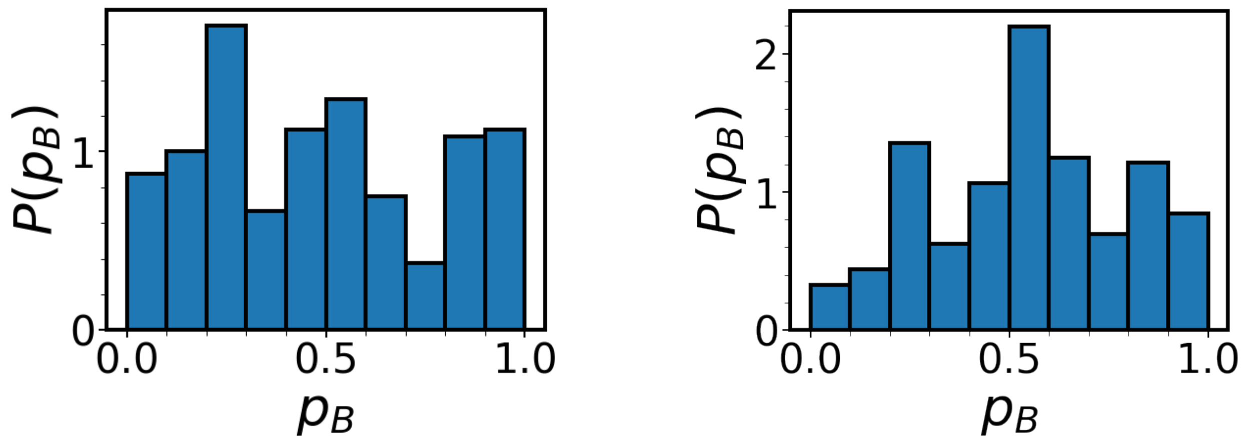


**(a)** Before   **(b)** After

**Supplementary Figure 11:** The probability distribution of the committor $p_B$ for the transition state ensemble identified by SPIB in the full system before (a) and after (b) including the "acceleration" OPs.

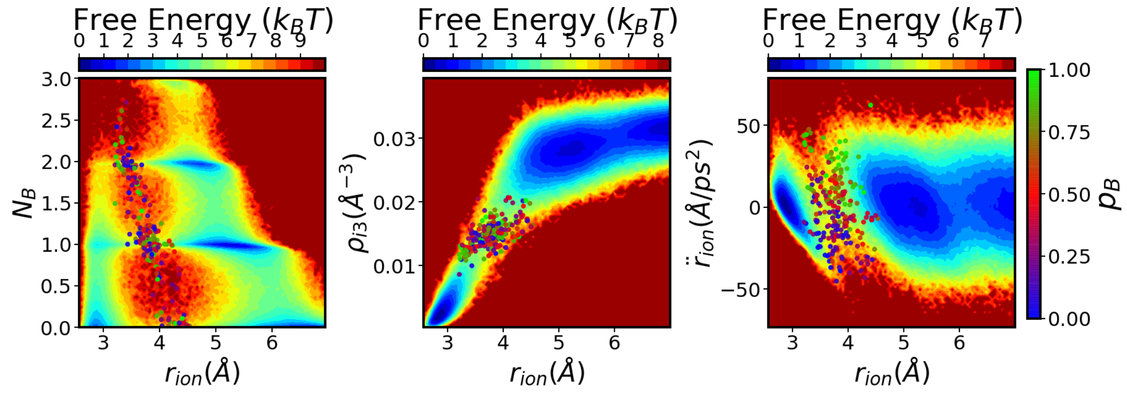


**Supplementary Figure 12:** Free energy projected onto coordinates $r_{ion}$ and $N_B$ (left), $r_{ion}$ and $\rho_{i3}$ (middle), and $r_{ion}$ and $\ddot{r}_{ion}$ (right) for the full system. Transition state ensembles identified by SPIB with the time delay $\Delta t = 0.4ps$ before including the "acceleration" OPs are projected onto each surface and colored according to their committor estimates $p_B$.

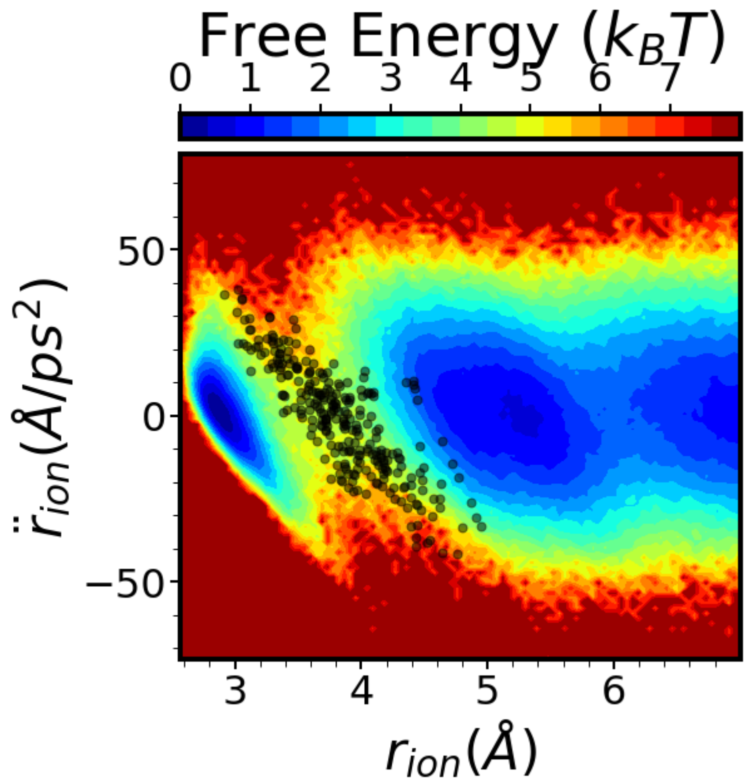


**Supplementary Figure 13:** Free energy projected onto coordinates $r_{ion}$ and $\ddot{r}_{ion}$ for the full system. The new Transition state ensemble identified by SPIB with the time delay $\Delta t = 0.4ps$ after including the "acceleration" OPs are projected onto the 2D surface as black points.

## VII. INPUT ORDER PARAMETER RELEVANCE ANALYSIS

In order to better interpret our RC, we adopt a method to approximately extract the information encoded in the nonlinear encoder by sequential randomization of input parameters.[13,14] To analyze the relevance of each input order parameter $X_j$ to the learned RC, we build the set $\{\tilde{\boldsymbol{X}}^i(j), \boldsymbol{y}^i\}$ by replacing the $j$-th input order parameter $X^i_j$ with a random number uniformly distributed between the extreme values of $X^i_j$ over the whole data set $X^i_j \sim \mathcal{U}(\min_i(X^i_j), \max_i(X^i_j))$. We then define the input relevance as the increase of the distortion due to the lost information of the $j$-th input order parameter by resampling:

$$r(X_j) = \sum_{n=1}^{N} \sum_{i=1}^{D} y_i^{n+s} \left[ \log \mathcal{D}_i(\boldsymbol{\mu}(\tilde{\boldsymbol{X}}^n(j)); \theta) - \log \mathcal{D}_i(\boldsymbol{\mu}(\boldsymbol{X}^n); \theta) \right]. \quad (11)$$

The larger this quantity is, the more informative $X_j$ is as an input order parameter. We normalize the input relevance by subtracting the converged distortion of the unperturbed

input data and dividing all entries by the largest relevance. We then rank each input coordinate $X_j$ by the normalized $r(X_j)$ and identified the most relevant ones.

In order to interpret the RC learned by SPIB with the time delay $\Delta t = 0.4\ ps$, we rank all the 13 input order parameters according to the increase in loss caused by their replacement with noise (Supplementary Fig. 14). The top two important order parameters are the ion-pair distance $r_{ion}$ and the number of bridging water molecules $N_B$, which are used to visualize the different metastable states learned by SPIB in the main text. The result illustrates that the learned RCs shared the same relevant components for different systems.

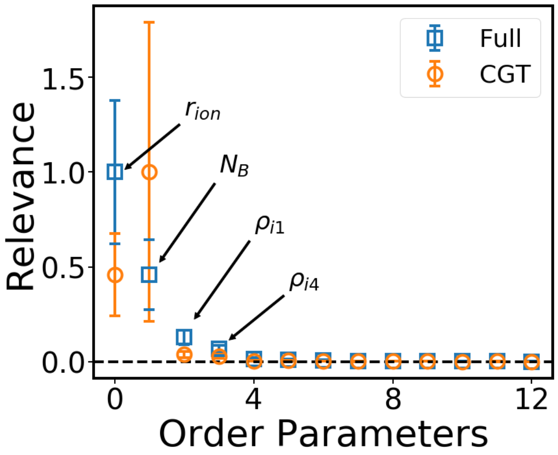


**Supplementary Figure 14:** Input relevance analysis of the learned RC for different systems. The input order parameters are ranked by their relevance in the full system. The standard deviations over 10 training runs are reported. The first order parameter $r_{ion}$ corresponds to the distance between the ion pair. The second order parameter $N_B$ corresponds to the number of bridging water molecules. The third and forth order parameters ($\rho_{i1}$ and $\rho_{i4}$) correspond to the interionic water density, which are similar to $\rho_{i3}$ just with different length resolution. (see Sec. II)

To better interpret the TSE, we extract all the samples near the transition states ($0.01\mathring{A}^{-3} < \rho_{i3} < 0.018\mathring{A}^{-3}$) for the input relevance analysis (shown in Supplementary Fig. 15). The top three relevant order parameters are the number of bridging water molecules $N_B$, interionic water density $\rho_{i4}$ and ion-pair distance $r_{ion}$, which are consistent with the report of Ref. 5. However, other OPs such as $N_{ip1}$ and $N_{Na,1}$ also seem to contribute to the identification of the transition state ensemble. The same top 3 OPs picked up by the three

systems are the same, suggesting that similar transition state ensembles are identified by SPIB.

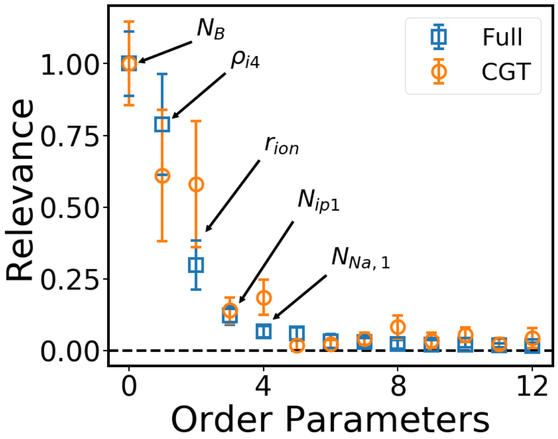


**Supplementary Figure 15:** Input relevance analysis of the learned RC near the transition states. The input order parameters are ranked by their relevance in the full system. The standard deviations over 10 training runs are reported. The forth order parameter $N_{ip1}$ corresponds to the total water molecules in the first shell of the ion pair. The fifth order parameter $N_{Na,1}$ corresponds to the coordination number in the first solvation shell of $Na^+$.

## SUPPLEMENTARY REFERENCES


[1] R. C. Remsing, J. M. Rodgers, and J. D. Weeks, Journal of Statistical Physics **145**, 313 (2011).

[2] S. Nosé, The Journal of chemical physics **81**, 511 (1984).

[3] S. Nosé and M. Klein, Molecular Physics **50**, 1055 (1983).

[4] J. M. Rodgers and J. D. Weeks, The Journal of chemical physics **131**, 244108 (2009).

[5] R. G. Mullen, J.-E. Shea, and B. Peters, Journal of chemical theory and computation **10**, 659 (2014).

[6] C. E. Shannon, IRE Nat. Conv. Rec **4**, 1 (1959).

[7] A. Alemi, B. Poole, I. Fischer, J. Dillon, R. A. Saurus, and K. Murphy, (2018).

[8] J. M. Tomczak and M. Welling, arXiv preprint arXiv:1705.07120 (2017).

[9] D. P. Kingma and M. Welling, arXiv preprint arXiv:1312.6114 (2013).

[10] D. P. Kingma and J. Ba, arXiv preprint arXiv:1412.6980 (2014).

[11]Y. Wang, J. M. L. Ribeiro, and P. Tiwary, Nature communications **10**, 3573 (2019).

[12]B. Peters, Chemical Physics Letters **554**, 248 (2012).

[13]S. J. Kemp, P. Zaradic, and F. Hansen, Ecological modelling **204**, 326 (2007).

[14]H. Jung, R. Covino, and G. Hummer, arXiv preprint arXiv:1901.04595 (2019).
